# Supplementary material for: Chiral and topological superconductivity in isospin polarized multilayer graphene
Source: arXiv:2409.13829 source file (2026-07-05)

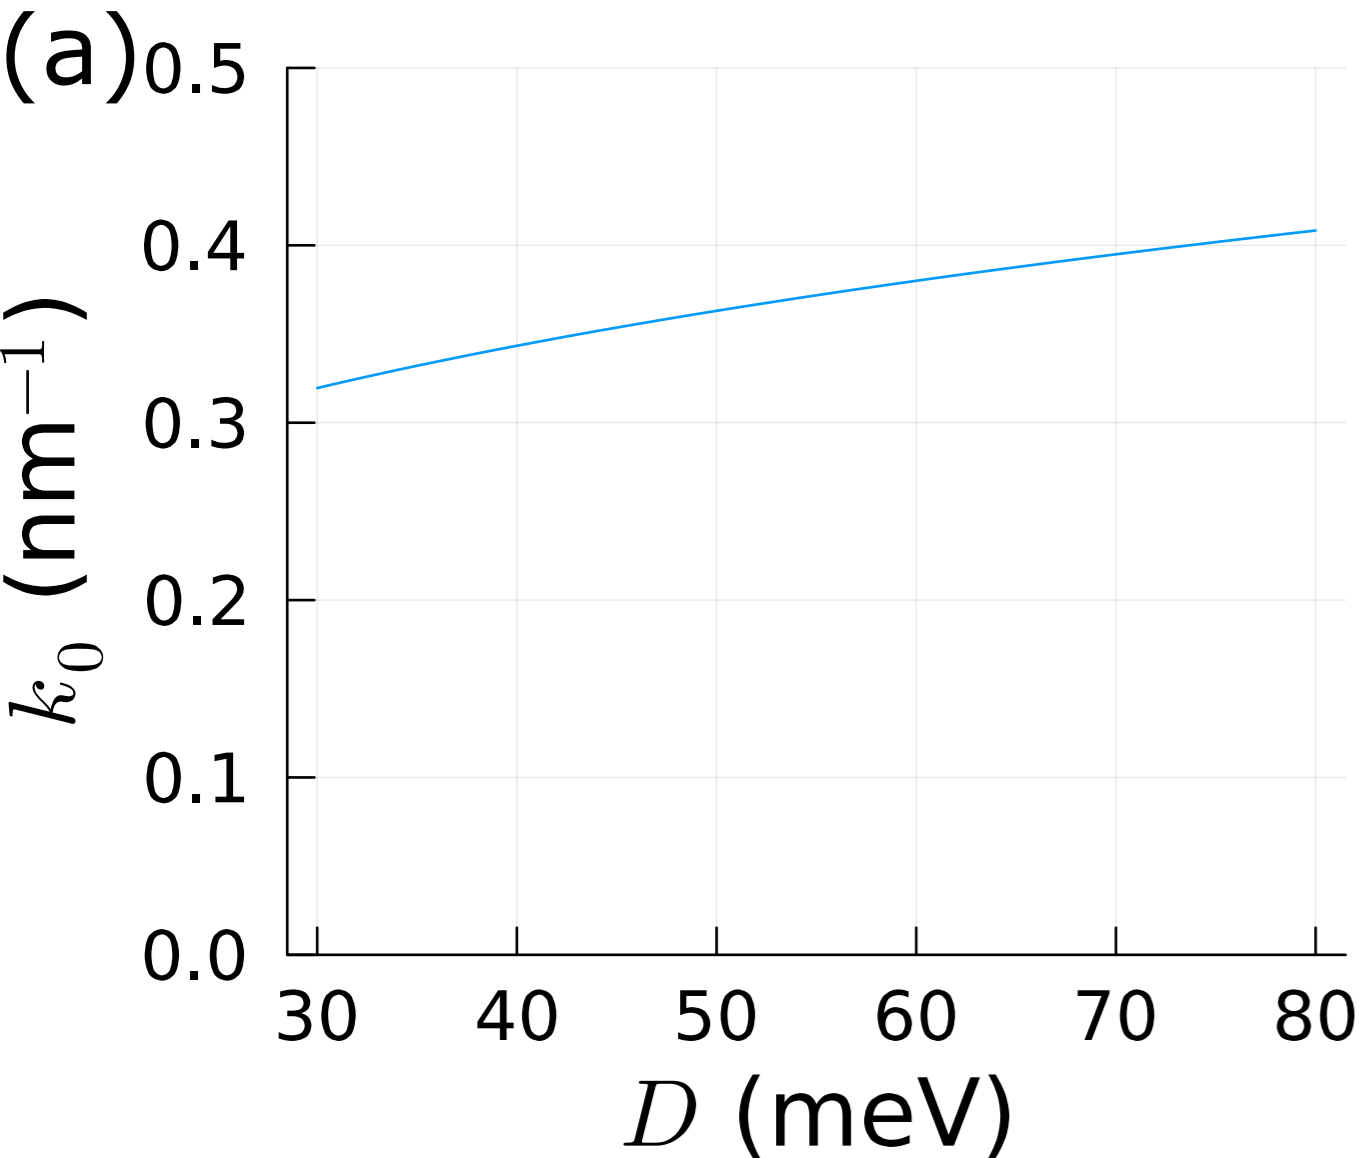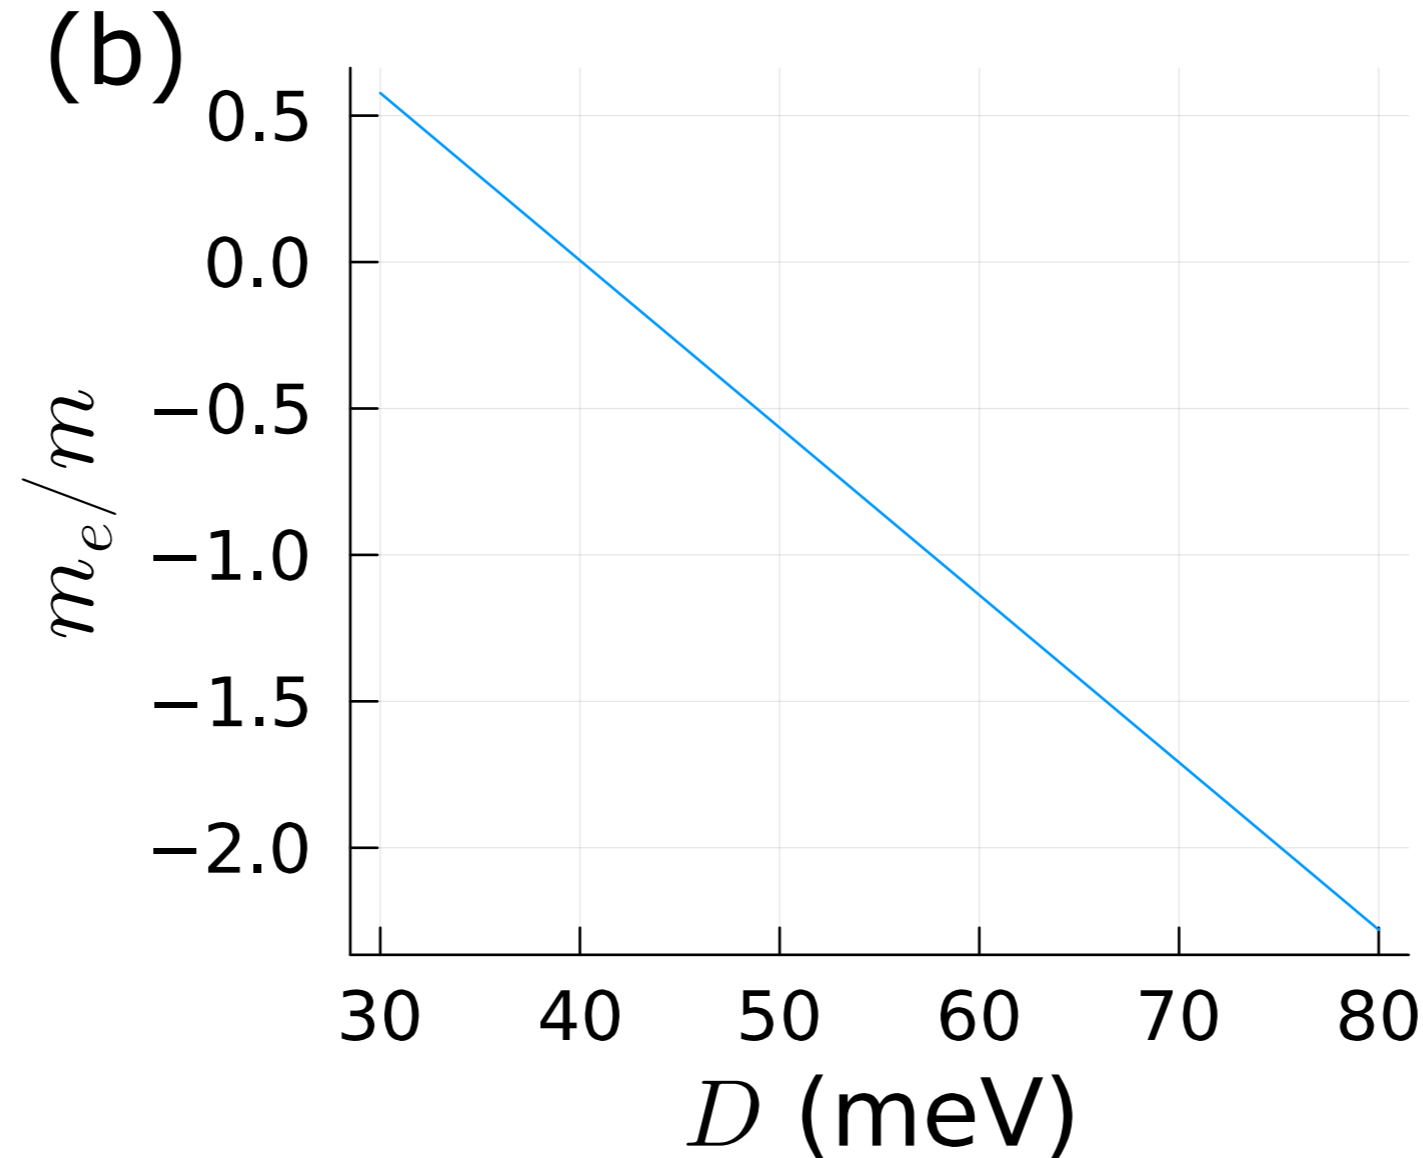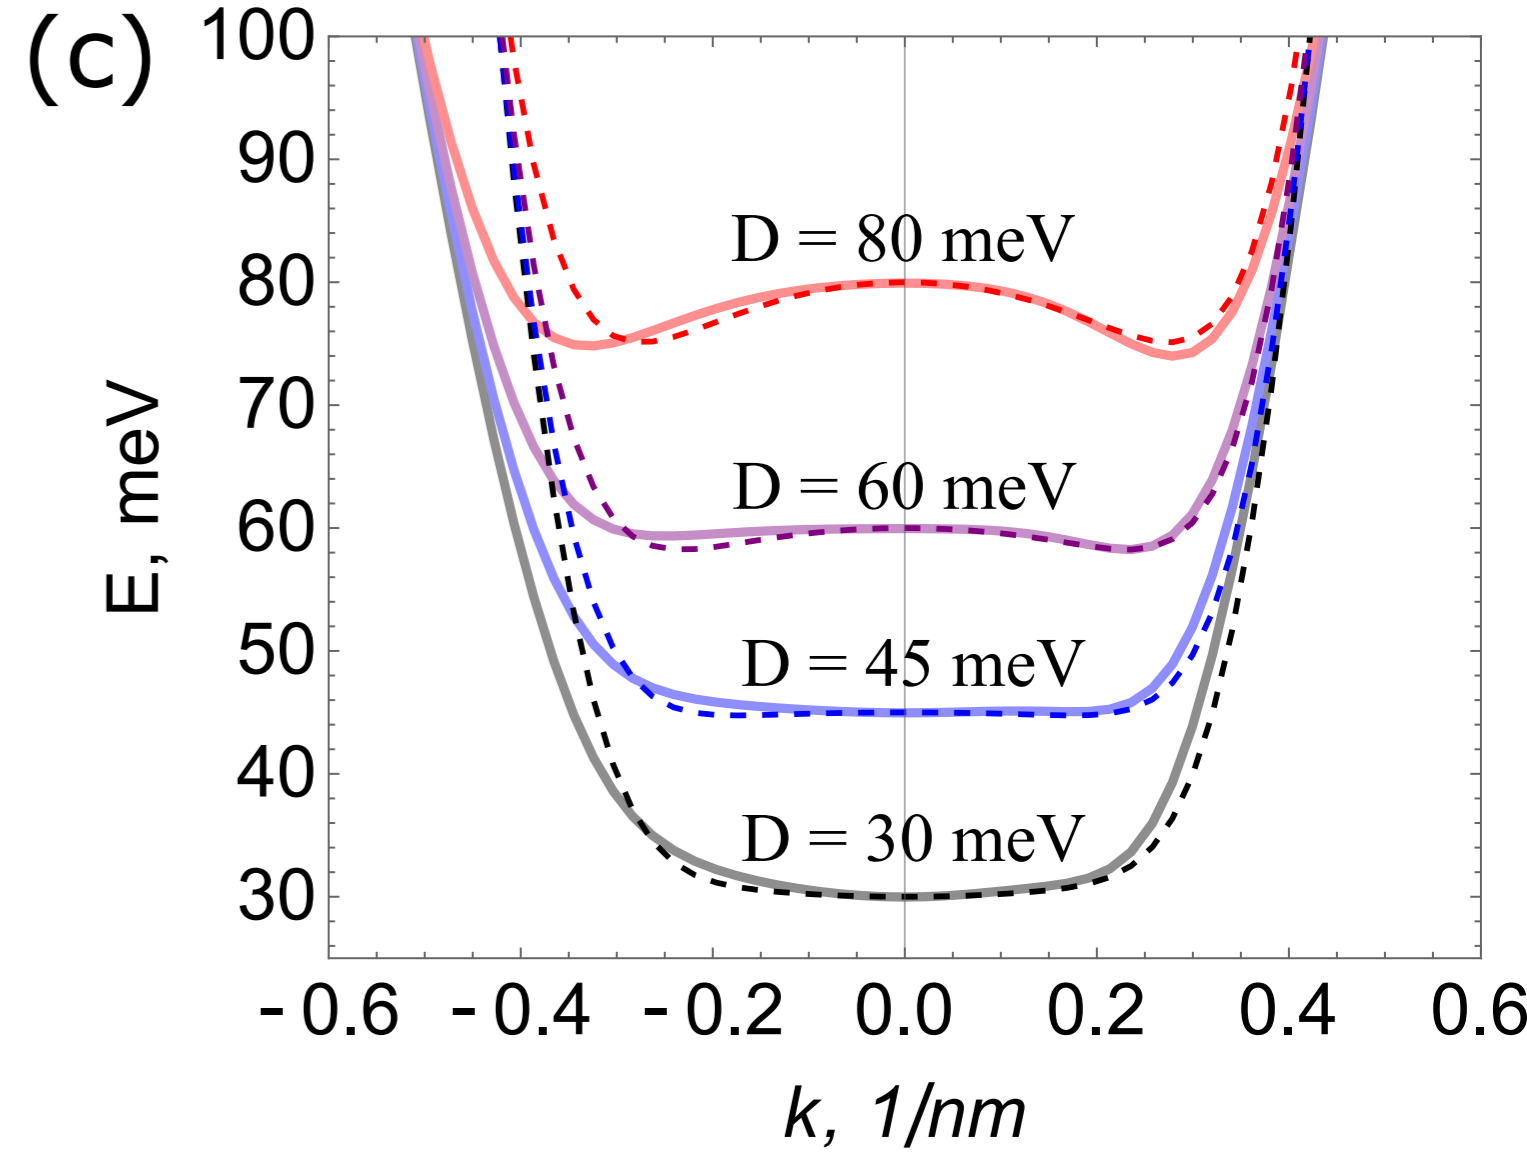

Supplement: Supplementary file 1 [file supp-FitsDispersion.pdf]
