# Supplementary material for: Chiral and topological superconductivity in isospin polarized multilayer graphene
Source: arXiv:2409.13829 source file (2026-07-05)

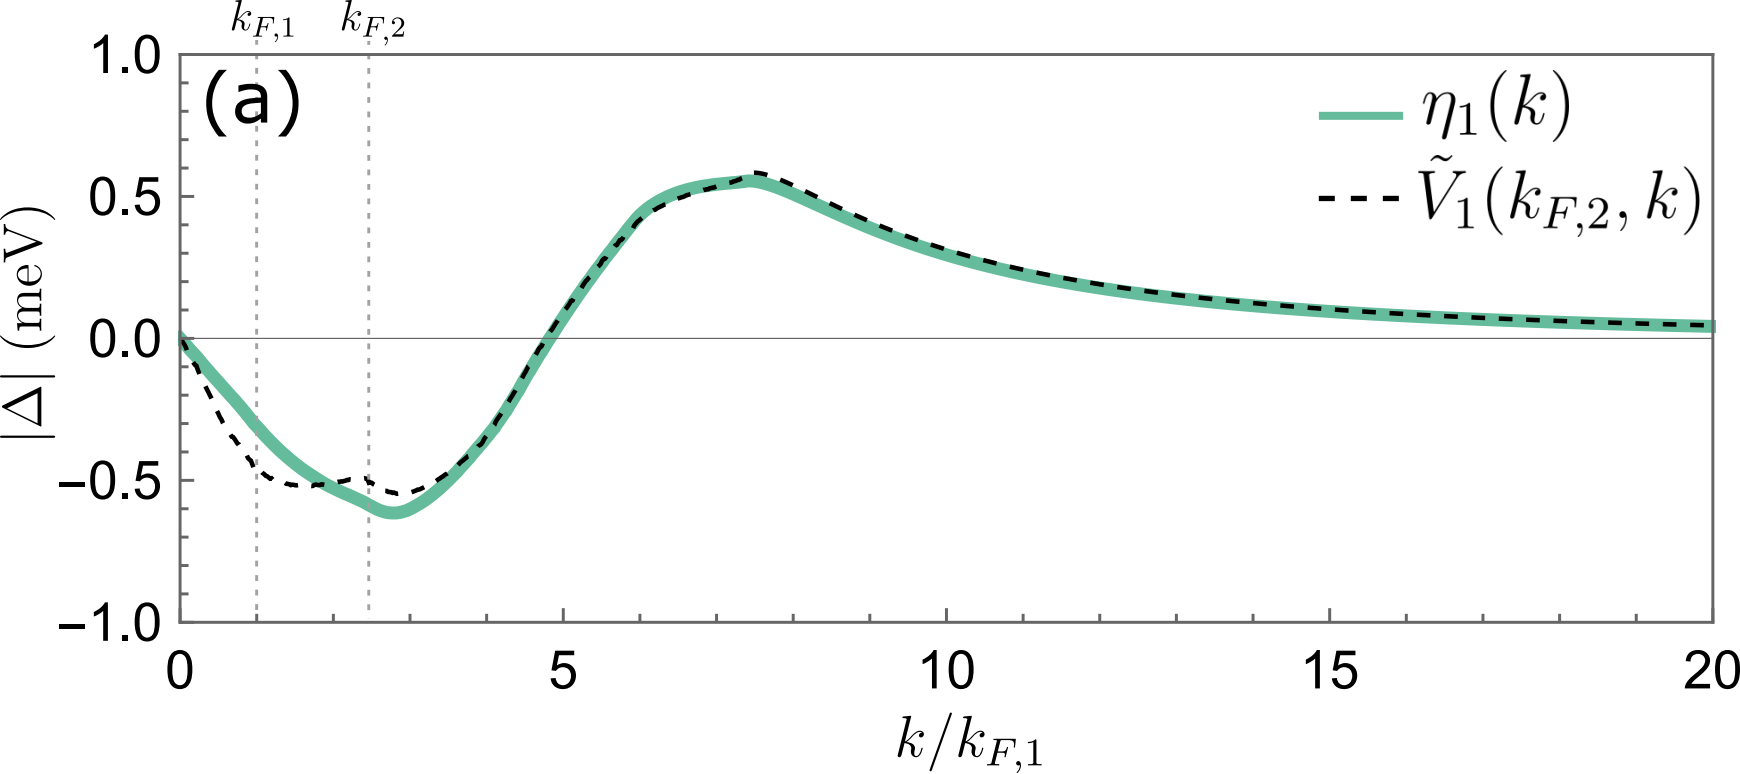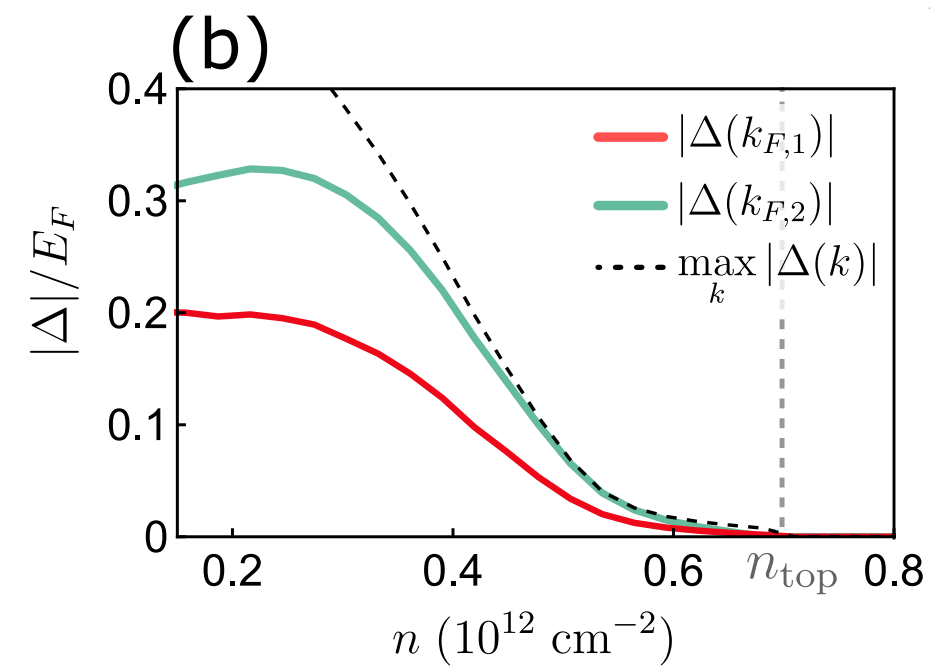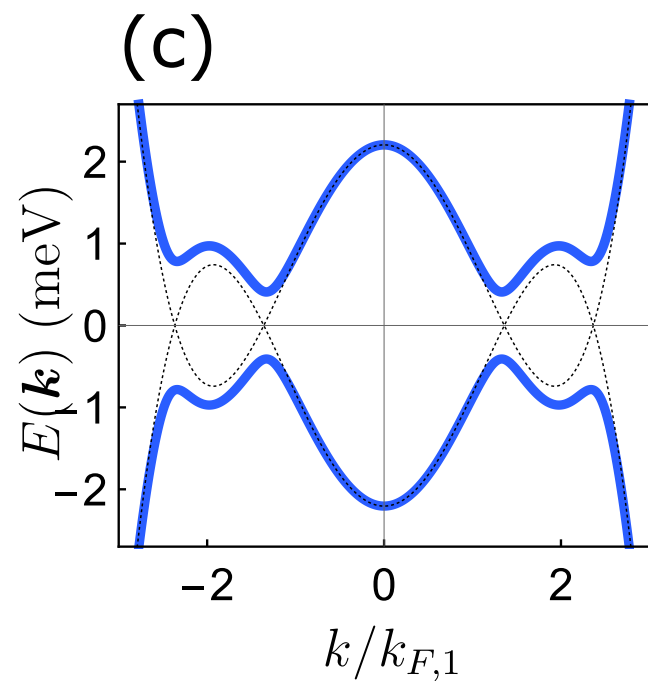











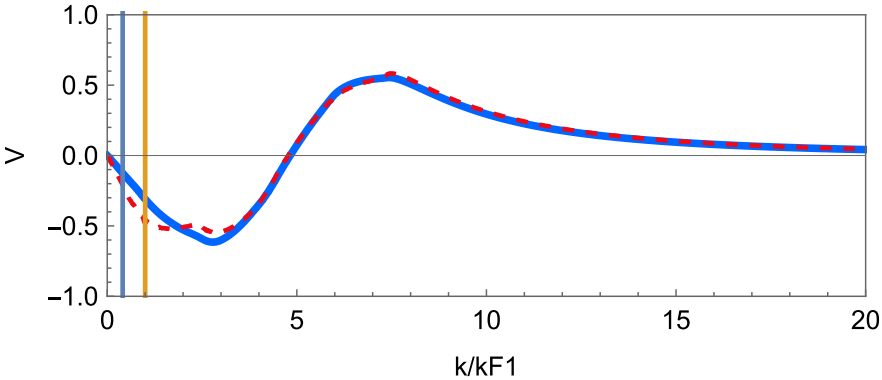

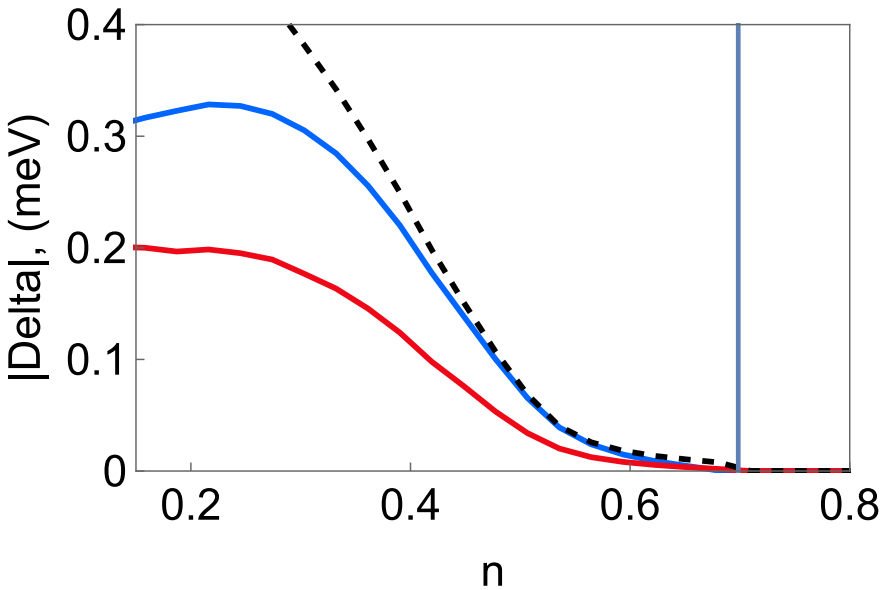

Supplement: Supplementary file 2 [file supp-fig4.1.pdf]
